# Supplementary material for: FB-4D: Spatial-Temporal Coherent Dynamic 3D Content Generation with Feature Banks
Source: arXiv:2503.20784 source file (2025-03-26)
Supplement: Supplementary file 1 [file X_supple.tex]

% \clearpage
% \setcounter{page}{1}
% \maketitlesupplementary

\section{LLM-Agents Details}
\subsection{Agent Implement Details}
LLM-Agents consist of their LLM (Large Language Model) component and corresponding functionalities. All experiments utilize the GPT-4 API\cite{llm_gpt4} to implement the LLM part. In each agent's prompt, there are elements involving the agent's function, the definition of actions that the agent needs to perform, the definition of information inputted to the agent, and the definition of outputs required from the agent. To facilitate the integration of Python code and ensure stable calls, the LLM part is required to return information in the format of a JSON dictionary. Additionally, each LLM part's prompt includes some examples, which contain inputs for certain scenarios and the corresponding expected outputs. If the input command does not contain the information of the keys of the output JSON dictionary, a default one will be filled in the dictionary. The parameters related to the GPT-4 API are all set to the official default values.

Note that, for supporting modification operations during multi-round commands, the 3D asset management agent, the vehicle motion agent, and the vehicle deleting agent have the ability to modify the information of already added or deleted cars.

\subsection{Reasoning Processes}
This section describes the natural language reasoning processes for the three cases presented in Section 5.2 of the main text.

\textbf{Mixed and complex command.} The initial input command is: \textit{"Remove all cars in the scene and add a Porsche driving the wrong way toward me fast. Additionally, add a police car also driving the wrong way and chasing behind the Porsche. The view should be moved 5 meters ahead and 0.5 meters above."} The command is decoupled by the project manager agent as following commands: 1.\textit{"Remove all cars."}; 2. \textit{"Add a Porsche driving the wrong way toward me fast."}; 3. \textit{"Add a police car also driving the wrong way and chasing behind the Porsche."}; 4. \textit{"The view should be moved 5 meters ahead and 0.5 meters above."}. The \textit{"Remove all cars."} command is distributed to the vehicle deleting agent, and then the agent finds the 3D boxes of all cars and applies the inpainting function for the removal operation. \textit{"Add a Porsche driving the wrong way toward me fast."} command is distributed to the 3D asset management agent for selecting the proper 3D asset. This command will also be distributed to the vehicle motion agent, which utilizes the key information in the command including "wrong way", "toward me" and "fast" to choose the appropriate start and end points and generate the motion with the motion generation function. \textit{"Add a police car also driving the wrong way and chasing behind the Porsche."} command will also be executed in the same way as the former operation. This command mentions the information of the added car, and the added car's information has been memorized by the project manager. This information is offered to the vehicle motion agent for determining the added police car's location. \textit{"The view should be moved 5 meters ahead and 0.5 meters above."} command is distributed to the view adjustment agent. The view adjustment agent returns the adjustment information of extrinsic as configuration, and calls the function to change the extrinsics to achieve view adjustment. Finally, background rendering and foreground rendering agents are required to generate the background and foreground results according to the information returned by the other agents, and the results are composed as the final outputs.

\textbf{Highly abstract command.} The initial input command is: \textit{"Create a traffic jam."} The project manager agent analyzes the command and decouples it as multiple repeats of car addition. These addition commands are processed by the 3D asset management agent and vehicle motion agent successively and are rendered by the foreground rendering agent. Combined with the rendered results from the background rendering agent, we can get the final outputs.

\textbf{Multi-round command.} The first initial command is: \textit{"Ego vehicle drives ahead slowly. Add a car to the close front that is moving ahead.”} The command is decoupled by the project manager agent as 1: \textit{"Ego vehicle drives ahead slowly."}; 2: \textit{"Add a car to the close front that is moving ahead."}. The first sub-command is distributed to view the adjustment agent, and the agent generates the extrinsics that represent moving ahead slowly. The second sub-command is executed as the process introduced above. 

The second initial command is: \textit{"Modify the added car to turn left. Add a Chevrolet to the front of the added car. Add another vehicle to the left of the added Mini driving toward me."} The command is decoupled by the project manager agent as 1: \textit{"Modify the added car to turn left."}; 2: \textit{"Add a Chevrolet to the front of the added car."}; 3: \textit{"Add another vehicle to the left of the added Mini driving toward me."} The first sub-command is distributed to the vehicle motion agent, which generates new motion based on the command for the determined added car. The following two sub-commands are executed in the same way as mentioned in the paragraphs above. Compositing the outputs of background rendering and foreground rendering agents can get the final outputs.

\section{Skydome Lighting Estimation Details}
\subsection{HDRI dataset}
We collect 449 high-quality outdoor panorama HDRIs from \href{https://polyhaven.com/hdris}{Poly Heaven Website}. These HDRIs are all licensed as CC0. We randomly selected 357 HDRIs for the training set and the remaining for the test set. A script for downloading these HDRIs will be available. 

\begin{figure*}[t]
    \centering
    \includegraphics[width=0.9\textwidth]{imgs/sup_skydome1.jpg}
        \vspace{-3mm}
    \caption{LDR to HDR reconstruction network. We add an explicit spherical Gaussian lobe encoded attenuation to overcome the over-smoothness in the decoded HDR panorama. It effectively ensures that the sun's intensity significantly exceeds that of surrounding pixels, rendering strong shadow effects for inserted objects. }
    \label{fig:ldr_to_hdr}
    \vspace{-3mm}
\end{figure*}

\begin{figure*}[t]
    \centering
    \includegraphics[width=0.9\textwidth]{imgs/sup_skydome2.jpg}
    \vspace{-3mm}
    \caption{Reconstructing HDR skydome from multi-camera images. Training on HoliCity~\cite{zhou2020holicity} dataset.}
    \vspace{-3mm}
    \label{fig:predict_from_mc}
\end{figure*}

\subsection{LDR to HDR Skydome Reconstruction}
In this step, we utilize our HDRI dataset to train an LDR to HDR autoencoder with the aim of converting the skydome into a compact feature representation. We use the sRGB opto-electronic transfer function (also known as gamma correction) to get the LDR sky panorama, and follow ~\cite{wang2022neural} to transform the LDR sky panorama to 3 intermediate vectors, including the sky content vector $\mathbf{f}_{\rm content} \in \mathbb{R}^{64}$, the peak direction vector $\mathbf{f}_{\rm dir} \in \mathbb{R}^{3}$ and the intensity vector $\mathbf{f}_{\rm int} \in \mathbb{R}^{3}_{+}$. In the process of converting intermediate vectors into a reconstructed HDR sky panorama, we construct the peak direction map \(\mathbf{M}_{\rm dir}\), the peak intensity map \(\mathbf{M}_{\rm int}\) and the positional encoding map \(\mathbf{M}_{\rm pe}\).

Peak direction map (\(\mathbf{M}_{\rm dir}\)): For each pixel in \(\mathbf{M}_{\rm dir}\), we calculate the peak direction embedding. This calculation utilizes a spherical Gaussian lobe, formulated as \(\mathbf{M}_{\rm dir}(\mathbf{u}) = e^{100*(\mathbf{u}\cdot \mathbf{f}_{dir} -1)}\), where \(\mathbf{f}_{\rm dir}\) denotes the peak direction vector. This map is represented in  \(\mathbb{R}^{H \times W \times 1}\).

Peak intensity map (\(\mathbf{M}_{\rm int}\)): Each pixel in this map is determined based on its corresponding value in the peak direction map. Specifically, for a given direction \(\mathbf{u}\), if \(\mathbf{M}_{\rm dir}(\mathbf{u}) > 0.9\), then \(\mathbf{M}_{\rm int}(\mathbf{u})\) is assigned the value of \(\mathbf{f}_{\rm int}\). If not, \(\mathbf{M}_{\rm int}(\mathbf{u})\) is set to zero. This map is represented in  \(\mathbb{R}_{+}^{H \times W \times 3}\).

Positional encoding map (\(\mathbf{M}_{\rm pe}\)): This map encodes the direction vector of each pixel, determined through equirectangular projection, thus contributing to the accurate reconstruction of the HDR sky panorama. It is defined in  \(\mathbb{R}^{H \times W \times 3}\).

The input of the decoder $\mathbf{M}_{\rm input}$ is a concatenation of $\mathbf{M}_{\rm pe}, \mathbf{M}_{\rm dir}$ and $ \mathbf{M}_{\rm int}$. We use a 2D UNet to decode the concatenated input map to the HDR sky panorama. For sky content vector $\mathbf{f}_{\rm content}$, we use an MLP to increase its feature dimension, reshape it to a 2D feature map, and concatenate it with the intermediate features at the bottleneck of the UNet. This concatenated feature will be further decoded to the HDR sky panorama.

In the context of HDR imaging, the intensity of the peak often exhibits characteristics akin to an impulse response, displaying pixel values that are significantly elevated by orders of magnitude in comparison to adjacent pixels. This presents a substantial challenge for the decoder in accurately recovering these patterns. Thus, we design a residual connection to explicitly inject the peak intensity information into the final HDR sky panorama. Let \(\mathbf{M}_{\rm peak}\) be the product of \(\mathbf{M}_{\rm dir}\) and \(\mathbf{M}_{\rm int}\), representing an attenuation encoded by a spherical Gaussian lobe. In our design, we specifically substitute the decoded HDR sky panorama at the peak position with \(\mathbf{M}_{\rm peak}\). This substitution is applied where the value of \(\mathbf{M}_{\rm int}(\mathbf{u})\) is non-zero, ensuring that the peak position in the HDR sky panorama is accurately represented by \(\mathbf{M}_{\rm peak}\). This makes a significant difference between us and ~\cite{wang2022neural}. Accurate and strong peak intensity can generate very strong shadow effects, resulting in better rendering realism. See Figure ~\ref{fig:ldr_to_hdr}.

To train the LDR to HDR skydome reconstruction, we computer the ground truth peak direction \(\mathbf{f}_{\rm dir}^{\rm gt}\) and peak intensity \(\mathbf{f}_{\rm int}^{\rm gt}\) from the HDR ground-truth. During the network training process, we employ four losses for supervision. These losses are as follows: 
peak direction loss $L_{\rm dir}$, which measures the L1 angular error of the peak direction vectors;
peak intensity loss $L_{\rm int}$, which quantifies the log-encoded L2 error of the peak intensity vectors;
HDR reconstruction loss $L_{\rm hdr-recon}$, which evaluates the log-encoded L2 error between the reconstructed HDR output and the ground truth HDR data;
LDR reconstruction loss $L_{\rm ldr-recon}$, which is calculated as the L1 error between the input LDR sky panorama and the gamma-corrected HDR reconstruction. 

The total loss is $L_{\rm total} = \lambda_1 L_{\rm dir} + \lambda_2 L_{\rm int} + \lambda_3 L_{\rm hdr-recon} + \lambda_4 L_{\rm ldr-recon}$, where $\lambda_1=1, \lambda_2=0.1, \lambda_3=2$ and $\lambda_4=0.2$. 

Data augmentation methods, including rotation, flipping, exposure adjustment and white balance adjustment, are implemented to enrich the training data. Noticing a strong white balance inaccuracy (the color temperature is too high) in the image data from Waymo Open Dataset~\cite{sun2020scalability}, we augment the HDRI with corresponding white balance adjustment. The blue channel is randomly enlarged by 1.2-1.3 times, and the red channel is randomly reduced by 1.2-1.3 times.

\subsection{Predict HDR Skydome from Multi-Camera Images}
This step involves estimating skydome lighting from multi-camera images collected by the vehicle. The core idea is to estimate intermediate features from multiple views and restore the skydome lighting using the well-trained HDR reconstruction decoding module. We emphasize the fusion of intermediate features from multiple cameras to get a complementary and comprehensive prediction for the skydome lighting.

Multi-camera image data will first go through a shared image encoder to predict the peak direction vector $\mathbf{f}_{\rm dir}^{(i)}$, the intensity vector $\mathbf{f}_{\rm int}^{(i)}$, and the sky content vector $\mathbf{f}_{\rm content}^{(i)}$ for each image $\mathcal{I}^{(i)}$, where $i$ is the camera index. For those vectors from $N$ cameras, we fuse all the features in the following strategy:

 We transform $\mathbf{f}_{\rm dir}^{(i)}, i=1,2,...,N$ to the front-facing view using their extrinsic parameters and averaged the rotated direction vector to $\bar{\mathbf{f}}_{\rm dir}$; we average $\mathbf{f}_{\rm int}^{(i)}, i=1,2,...,N$ to $\bar{\mathbf{f}}_{\rm int}$; we utilize the attention mechanism to fuse sky content vectors as $\bar{\mathbf{f}}_{\rm content} = \texttt{Attn(q, k, v)}$, where $\texttt{q} = \mathbf{f}^{(0)}_{\rm content}$, $\texttt{k} =\texttt{v} = \texttt{stack} (\{\mathbf{f}^{i}_{\rm content}\}_{i=0,1,...,N-1})$. Here index 0 refers to the first (front-facing) view image and $\texttt{Attn}(\cdot,\cdot,\cdot)$ the standard attention operator. Given $\bar{\mathbf{f}}_{\rm dir}$, $\bar{\mathbf{f}}_{\rm int}$, $\bar{\mathbf{f}}_{\rm content}$, we use the pre-trained decoding module from the previous stage to recover the fused intermediate vectors to HDR panorama. See Figure ~\ref{fig:predict_from_mc}.

Since there is no relevant panoramic data in the autonomous driving dataset for supervision, We use HoliCity~\cite{zhou2020holicity} to simulate multi-camera images.  Based on the arrangement and FOV of the three forward-facing cameras on the Waymo vehicle~\cite{sun2020scalability}, we cropped the corresponding image from the HoliCity panorama as the model inputs. To supervise the learning of the image encoder, we use the LDR to HDR reconstruction network from the previous stage to generate pseudo peak intensity vector GT, peak direction vector GT, sky content vector GT, and HDR skydome GT. 

We apply five losses to supervise the network during training. These losses are as follows: the peak direction loss $L_{\rm dir}$, which measures the L1 angular error of the fused peak direction vector; the peak intensity loss $L_{\rm int}$, which calculates the log-encoded L2 error of the fused peak intensity vectors; the sky content loss $L_{\rm content}$, which evaluates the L1 error of the fused sky content vectors; the HDR reconstruction loss $L_{\rm hdr-recon}$ with log-encoded L2 error; the LDR reconstruction $L_{\rm ldr-recon}$ with L1 error. 

The total loss is $L_{\rm total} = \lambda_1 L_{\rm dir} + \lambda_2 L_{\rm int} + \lambda_3 L_{\rm content} + \lambda_4 L_{\rm hdr-recon} + \lambda_5 L_{\rm ldr-recon}$, where $\lambda_1=0.5, \lambda_2=0.25, \lambda_3=0.005, \lambda_4=0.1$ and $\lambda_5=0.2$.

\section{3D Asset Bank}
To ensure ease of access and modification of 3D assets, we normalize our Blender models within their Blender files using the following procedure:

\begin{enumerate}
    \item We ensure that the model has accurate physical dimensions in the unit of meter.
    
    \item The origin of the car model is set at the middle of the bottom of the car. We position the model at the center of the world coordinate system, ensuring that the car model's origin aligns with the origin of the world coordinate system. The car is oriented to face the positive direction of the x-axis.

    \item We uniformly apply the \texttt{Principled BSDF} material to the car body, and name the material "car\_paint". Prompt that changes the asset's color will affect the "Base Color" attribute of the \texttt{Principled BSDF} node.

    \item We use the \texttt{Join} operator to merge all meshes into one object. 

\end{enumerate}

Following the aforementioned approach, we normalize the Blender models collected from the Internet to continuously expand our 3D Asset Bank.

\section{Blender Rendering Details}
We fully implement the Blender rendering workflow using Python scripting, incorporating features such as alpha channel, depth channel, and shadow effect, \textbf{all achieved within a single rendering pass}.

\begin{enumerate}
    \item To get a transparent background, we first enable the \texttt{Render Properties - Film - Transparent} option.
    \item To get multiple rendering output, we enable the \texttt{Combined} pass, \texttt{Z} pass and \texttt{Shadow Catcher} pass in \texttt{View Layer Properties} panel.
    \item To render the shadow, we add a very large plane under the car and enable the plane's \texttt{Object Properties - Visibility - Mask - Shadow Catcher} option. 
    \item To obtain scene-related colored shadows, we construct the compositing node graph as Figure ~\ref{fig:blender}. This configuration generates the rendered image overlaid on the scene image, along with the accompanying depth information and mask of the vehicle and its corresponding shadow.
    \begin{figure}[t]
        \centering
        \includegraphics[width=\columnwidth]{imgs/blender_node.jpeg}
            \vspace{-3mm}
        \caption{Compositing node graph design in Blender~\cite{blender}}
        \label{fig:blender}
            \vspace{-3mm}
    \end{figure}
    \item Using depth information and mask, we can handle the occlusion relationship with the original objects in the scene. We also added a moderate amount of motion blur to the rendered car to match the background.
\end{enumerate}

\section{Motion Generation Details}
The vehicle motion agent creates the initial places and subsequent motions of vehicles following the requests commands. Existing vehicle motion generation methods cannot directly generate motion purely from text and the scene map. Here we elaborate on the details of our text-to-motion methods. Our method consists of two parts: 
vehicle placement to generate the starting points and vehicle motion planning to generate the subsequent motions.

\begin{figure}
    \centering
    \includegraphics[width=0.38\textwidth]{imgs/supp_placement.png}
    \caption{The neighboring area division for vehicle placement.}
    \label{fig:vehicle_placement}
    \vspace{-3mm}
\end{figure}

\subsection{Vehicle Placement}
We use the language command and the scene map to generate the initial position. The scene map $\mathcal{M}$ follows the lane map form $\mathcal{M}=\{\mathbf{n}_i,i=1,2,\cdots,m\}$, where $m$ is the number of lane nodes and the $i$th lane node $\mathbf{n}_i=(x_{\rm s},y_{\rm s},x_{\rm e},y_{\rm e},c_{\rm type})$ consists of lane starting position $(x_{\rm s},y_{\rm s})$, ending position $(x_{\rm e},y_{\rm e})$ and the lane type $c_{\rm type}$. The map range is cropped with the range of front 80m, left 20m and right 20m. Generally, we use the lane map from the ground-truth data. If the lane map does not exist, it is applicable to use a lane map estimation method like \cite{liao2022maptr,liao2023maptrv2} to obtain the lane map. 

Given the language command, the LLM first extracts key placement attributes, including vehicle number, distance range, relative direction with the observer and direction of driving, and crazy mode. With these attributes, the role function of placement begins to find suitable lane nodes from the scene map. Here we assume all the placed vehicles are on the centerline of the road. If the distance range $(d_{\rm min},d_{\rm max})$ is identified, the role function selects the lane centerline nodes according to their distance with the ego location. For the relative direction, we divide the ego neighboring area into 6 categories: front, left front, right front, left, right, and back, see Figure~\ref{fig:vehicle_placement} for illustration. For the direction of driving, we consider two types: driving close to the ego and driving away from the ego, which determines the left/right side of the vehicle on the road. The crazy mode, which is designed for non-compliant inverse driving behavior, is a bool variable. When it is true, we will inverse the direction of the map (swap the starting and ending point of each lane) for that vehicle to represent inverse driving. We select the matched lane node set and randomly select one lane node from the set. We also consider the conflict of placing vehicles by an iterative approach that incoming vehicles should not overlap with the existing vehicles. After obtaining lane nodes for every vehicle, we set the midpoint of the lane node to be the initial position of a vehicle and the direction of the lane to be the initial heading of the vehicle.

\subsection{Vehicle Motion Planning}
After obtaining the initial positions, we generate motions in two steps: plan the destination and plan the middle trajectory. We first extract movement attributes including speed, action, interval and time length. Notably, we divide actions into 5 categories: straightforward, turn left, turn right, park, and backward.  
To obtain the destination, if the action category is straightforward or park, and backward, we directly calculate a raw destination by assuming the car driving following a line with the target speed. Then we find the closest lane node with the raw destination to be the final destination.
If the action category is turning left or turning right, we select a set of nodes whose vertical distance with the initial line of heading is in a range (5m-30m) and fit the driving directions (the direction of the line should be away from the starting point). We randomly pick a lane node to be the destination. 

To plan the middle trajectory, we use an iterative adjustment approach to make the trajectory match with the map and avoid off-road driving. We first use one cubic Bezier curve to fit the overall trajectory with the condition of starting point, starting direction, ending point and ending direction. The cubic Bezier curve is formulated by
\begin{equation}
\begin{aligned}
    B(t) = & (1-t)^3P_0 + 3t(1-t)^2P_1 \\
    &+ 3t^2(1-t)P_2 + t^3P_3, t\in [0,1], 
\end{aligned}
\end{equation}
where $P_0,P_1,P_2,P_3 \in \mathbb{R}^2$ is the control points that can be solved by given starting point, starting direction, ending point and ending direction. Then to avoid off-road driving of the intermediate trajectory, we adjust the middle coordinate by replacing it with the closest lane node. We split the whole trajectory into two parts with the boundary of the middle coordinate and use one cubic Bezier curve to fit each split trajectory. We iteratively repeat the process to represent the planned trajectory by multiple cubic Bezier curves. Finally, to make the planned trajectory fit with vehicle dynamics, we use a trajectory tracking method in \cite{xu2023drl} as post-processing to revise the planned trajectory.

\section{Background rendering details}
\subsection{Dataset Selection}
For all Waymo Open Dataset~\cite{sun2020scalability} experiments, we use images captured from three frontal cameras. The details of selection are shown in Table~\ref{dataset}. There are 120 images in total for each scenerio.

\begin{table}[]
\centering
\scriptsize
\begin{tabular}{c|c}
\toprule
Sequence & Start Frame \\
\midrule
segment-10247954040621004675\_2180\_000\_2200\_000 & 0 \\
segment-13469905891836363794\_4429\_660\_4449\_660 & 40 \\
segment-14333744981238305769\_5658\_260\_5678\_260 & 40 \\
segment-1172406780360799916\_1660\_000\_1680\_000 & 50 \\
segment-4058410353286511411\_3980\_000\_4000\_000 & 90 \\
segment-10061305430875486848\_1080\_000\_1100\_000 & 30 \\
segment-14869732972903148657\_2420\_000\_2440\_000 & 0 \\
segment-16646360389507147817\_3320\_000\_3340\_000 & 0 \\
segment-13238419657658219864\_4630\_850\_4650\_850 & 0 \\
segment-14424804287031718399\_1281\_030\_1301\_030 & 60 \\
segment-15270638100874320175\_2720\_000\_2740\_000 & 60 \\
segment-15349503153813328111\_2160\_000\_2180\_000 & 100 \\
segment-15868625208244306149\_4340\_000\_4360\_000 & 110 \\
segment-16608525782988721413\_100\_000\_120\_000 & 10 \\
segment-17761959194352517553\_5448\_420\_5468\_420 & 0 \\
segment-3425716115468765803\_977\_756\_997\_756 & 0 \\
segment-3988957004231180266\_5566\_500\_5586\_500 & 0 \\
segment-9385013624094020582\_2547\_650\_2567\_650 & 130 \\
segment-8811210064692949185\_3066\_770\_3086\_770 & 30 \\
segment-10275144660749673822\_5755\_561\_5775\_561 & 0 \\
segment-10676267326664322837\_311\_180\_331\_180 & 100 \\
segment-12879640240483815315\_5852\_605\_5872\_605 & 20 \\
segment-13142190313715360621\_3888\_090\_3908\_090 & 0 \\
segment-13196796799137805454\_3036\_940\_3056\_940 & 70 \\
segment-14348136031422182645\_3360\_000\_3380\_000 & 140 \\
segment-15365821471737026848\_1160\_000\_1180\_000 & 0 \\
segment-16470190748368943792\_4369\_490\_4389\_490 & 0 \\
segment-11379226583756500423\_6230\_810\_6250\_810 & 0 \\
segment-13085453465864374565\_2040\_000\_2060\_000 & 110 \\
segment-14004546003548947884\_2331\_861\_2351\_861 & 0 \\
segment-15221704733958986648\_1400\_000\_1420\_000 & 70 \\
segment-16345319168590318167\_1420\_000\_1440\_000 & 0 \\
\bottomrule
\end{tabular}
            \vspace{-3mm}
\caption{\small  Information on the selected and trimmed Waymo Open Dataset~\cite{sun2020scalability}. For each sequence, we select 40 frames starting from the Start Frame.  }
\label{dataset}
    \vspace{-3mm}
\end{table}

\begin{figure}
\centering 
\includegraphics[width=0.47\textwidth]{imgs/supp_compare.png} 
\vspace{-3mm}
\caption{\small Qualitative ablation of background rendering. (a) McNeRF w/o pose alignment.(b) McNeRF w/o exposure. (c) Full McNeRF. Last row: target images.}
\label{Fig:ablation} 
\vspace{-3mm}
\end{figure}

\subsection{Multi-Camera Alignment}
This section will introduce the details of our multi-camera alignment algorithm. Let $R_{C_i, t}$ and $T_{C_i, t}$ represents the camera $C_i$'s extrinsic matrix that aligned to vehicle's coordinates at timestamp $t$. $C_0$ is the front camera. The superscript $(V)$ and $(M)$ represents the original vehicle's coordinates in autonomous driving dataset and the coordinates under Metashape's unified space. Then the rotation $R_{C_i, t}$ and translation $T_{C_i, t}$ can be calculated as:
\begin{align*}
R_{C_i, t} &= R^{(V)}_{C_0, 0} (R^{(M)}_{C_0, 0})^{-1} R^{(M)}_{C_i, t} \\
T_{C_i, t} &= \frac{R^{(V)}_{C_0, 0} (R^{(M)}_{C_0, 0})^{-1} (T^{(M)}_{C_i, t} - T^{(M)}_{C_0, 0})}{S} + T^{(V)}_{C_0, 0}, \\
\end{align*}
where $S=\frac{T^{(M)}_{C_0, 1} - T^{(M)}_{C_0, 0}}{T^{(V)}_{C_0, 1} - T^{(V)}_{C_0, 0}}$ is a scaling factor that ensures the aligned space has the same unit length as the real world.

\section{Supplymentary Experiments}

\subsection{Qualitative Ablation Study of Background Rendering}
Figure \ref{Fig:ablation} illustrates the effects of the ablation study on background rendering. It is evident that in the absence of pose adjustment, the rendered results exhibit significant blur and anomalies. Without the intervention of exposure adjustments, there are noticeable changes in brightness at the junctions of different cameras, particularly in the sky. McNeRF, however, successfully avoids these two issues and achieves the optimal rendering outcomes.

\begin{figure*}
\centering 
\includegraphics[width=0.99\textwidth]{imgs/supp_occlusion.png} 
\vspace{-3mm}
\caption{\small Qualitative result of occlusion postprocess and the color control for added car.}
\label{Fig:occlusion} 
\end{figure*}
\subsection{Occlusion with Depth Test}
During the process of adding vehicles, there may be instances of occlusion. For occlusions among multiple vehicles to be added, Blender considers this issue during the rendering process. Therefore, we only need to focus on the occlusion between the foreground vehicles and the background objects. The most straightforward method to handle occlusion is determined by the depth map of the foreground and background, respectively. The depth maps of both the foreground and background could be used to choose for each pixel with the lesser depth to be displayed in the front, while the one with greater depth is occluded. However, accurately estimating the background's depth map directly is challenging. The point cloud data in autonomous driving datasets is too sparse, and the depth maps obtained through depth completion are also sparse and excessively noisy, making them unsuitable for pixel-level accuracy in practical use. Here, we combine the sparse depth data from point clouds with the object segmentation method SAM\cite{kirillov2023segment}. SAM can achieve pixel-level accuracy in segmentation results at the image level, without extra finetuning. We first use SAM to obtain different patches in the background image, then identify patches that overlap with the foreground objects. Using the sparse depth map derived from the point clouds, we calculate the average sparse depth within these patches as the depth of each patch. Since the segmentation results of patches often represent a complete instance, and occlusion occurs between instances, it is reasonable to calculate the depth for the entire instance represented by a patch. Subsequently, we create the background's depth map from the depths of these patches and perform occlusion calculations with the depth map rendered for the foreground, presenting each pixel with the lesser depth to finalize the occlusion computation. The results of the occlusion calculation, as shown in Fig. \ref{Fig:occlusion}, illustrate that the added vehicles are occluded by those with shallower depths. This figure also displays the adjustment of the added vehicles' colors.

\begin{figure*}
\centering 
\includegraphics[width=0.99\textwidth]{imgs/supp_obstacles.png} 
\vspace{-3mm}
\caption{\small Qualitative results of rare cases simulation.}
\label{Fig:obstacles} 

\end{figure*}

\subsection{Rare Cases Simulation}
Leveraging diverse external digital assets, ChatSim can simulate rare and challenging-to-collect real-world scenarios within reconstructed existing scenes. Figure \ref{Fig:obstacles} demonstrates ChatSim's ability to emulate rare cases by placing uncommon elements like bulldozers, isolation piers, fences, excavators, and other infrequently encountered situations in reconstructed scenes. This capability enables ChatSim to create rare digital twins for existing collected data, thus fulfilling the need for these specific scenarios.

\begin{table}[]
\centering
\begin{tabular}{c|ccc}
\toprule
Simulation data & AP30            & AP50            & AP70            \\ \hline
            0               & 0.1263          & 0.0366          & 0.0034       \\
            600             & 0.1910          & 0.0878          & 0.0153       \\
            1000            & \textbf{0.2074} & \textbf{0.0930} & \textbf{0.0189} \\
            2200            & 0.2064          & 0.0900          & 0.0182      \\ 
            \hline
\end{tabular}
            \vspace{-3mm}
\caption{Comparison of detection model’s performance with different number of data simulated by ChatSim}
\label{tab:augmentation_2}
\vspace{-3mm}
\end{table}

\subsection{Supplementary 3D Detection Augmentation Experiment}

We conducted 3D detection augmentation experiments under a new setting: we fixed the real data amount from the original dataset at 4200 frames and augmented it with varying quantities of simulation data generated by ChatSim. We continued to use Lift-Splat~\cite{philion2020lift} as the detection model, with results shown in Table \ref{tab:augmentation_2}. It is observed that the use of simulation data significantly enhances the performance of the 3D detection task. As the amount of simulation data increases, the final performance tends to stabilize after a certain point of improvement.

% \section{User Study Details}
% \textbf{Motion experiment user study.} We generate 35 different motions for our motion generation method and the two baselines with specific action control and visualize the motion and map. The 12 users are required to judge if the visualization of motion satisfies the action and if the motion is within the road boundary. 
